# Supplementary material for: User Agency and System Automation in Interactive Intelligent Systems
Source: arXiv:2502.13779 source file (2025-02-19)
Supplement: Supplementary file 1 [file 90_appendix.tex]

\appendix
