# Supplementary material for: User Agency and System Automation in Interactive Intelligent Systems
Source: arXiv:2502.13779 source file (2025-02-19)
Supplement: Supplementary file 2 [file 99_appendix.tex]

\section{Control Algorithm}
\label{ap:control_algorithm}
\SetKwProg{Fn}{Function}{}{}
\begin{algorithm}[h]
\SetAlgoLined
\DontPrintSemicolon
 \Fn{MPCC($\mathbf{x0}, \mathbf{w},\posp, \mathbf{parameters}$)}{
 $[\mathcal{C}_l, \mathcal{C}_c, \mathcal{C}_\theta, \mathcal{C}_{\dot{\theta}}]\leftarrow$compute lag and contour error \;
 $[\mathcal{C}_f, \mathcal{C}_d, \mathcal{C}_\alpha]\leftarrow$compute force error \;
 $J_k \leftarrow $ sum($\mathcal{C}_l, \mathcal{C}_c, \mathcal{C}_\theta, \mathcal{C}_{\dot{\theta}},\mathcal{C}_f, \mathcal{C}_d, \mathcal{C}_\alpha$)\;
 $[\mathbf{x}, \mathbf{u}]\leftarrow$minimize($J_k$) \;
 }
  \Return $[\mathbf{x}, \mathbf{u}]$\;
  \;
 
 $\mathbf{x_0}$, $\mathbf{w} \leftarrow \ $initialize\;
\While{drawing not finished}{
  $\posp \leftarrow$ Measure pen position\;
  ${\posp}_{,k} \leftarrow$ $KalmanFilter(\posp) $\;
  $\mathbf{x_0} \leftarrow$ update system states, from sensor data\;
  $\mathbf{parameters} \leftarrow$ update MPCC parameters \;
  $[\mathbf{x_{t=1..n}},\mathbf{u_{t=1...n}}] \leftarrow$ $MPCC(\mathbf{x_0},\mathbf{w},\mathbf{p},\mathbf{params})$\;
  $\mathbf{x_0}\leftarrow \mathbf{x_1}$\;
  apply($\mathbf{u_0})$
 }
 \caption{Closed Loop Haptic Feedback Control.} 
\label{alg:optimization-overview}
\end{algorithm}

%%%%%I commented out the include statement for the entire appendix in Main.tex because of compilation errors. Undo that once you fixed the LAtex
